# Supplementary material for: Dynamic Mini-batch SGD for Elastic Distributed Training: Learning in the Limbo of Resources
Source: arXiv:1904.12043 source file (2019-05-02)
Supplement: Supplementary file 1 [file supplementary.tex]

%auto-ignore

\documentclass[10pt,twocolumn,letterpaper]{article}

\usepackage{iccv}
\usepackage{times}
\usepackage{epsfig}
\usepackage{graphicx}
\usepackage{amsmath}
\usepackage{amssymb}
\usepackage{epsfig}
\usepackage{graphicx}
\usepackage{amsmath}
\usepackage{amssymb}

\usepackage{graphicx}

\usepackage{microtype}
\usepackage{graphicx}
\usepackage{subfig}
\usepackage{booktabs} % for professional tables

\usepackage{algpseudocode}

\usepackage{amsthm}

\usepackage{nicefrac}
\usepackage{comment}
\usepackage{adjustbox}
\usepackage{arydshln}
\usepackage{lastpage}
\usepackage[T1]{fontenc}

\usepackage{algorithm}
%\usepackage{algorithmic}
%\usepackage[]{algorithm2e}

% Include other packages here, before hyperref.

% If you comment hyperref and then uncomment it, you should delete
% egpaper.aux before re-running latex.  (Or just hit 'q' on the first latex
% run, let it finish, and you should be clear).
\usepackage[breaklinks=true,bookmarks=false]{hyperref}

% \iccvfinalcopy % *** Uncomment this line for the final submission

 % *** Enter the ICCV Paper ID here

% Pages are numbered in submission mode, and unnumbered in camera-ready
%\ificcvfinal\pagestyle{empty}\fi
\setcounter{page}{1}
\begin{document}

%%%%%%%%% TITLE
\title{
Supplementary Material for Dynamic Stochastic Gradient Descent for Elastic Distributed Training: Learning in the Limbo of Resources
}

\author{}

\maketitle

\input{appendix.tex}

{\small
\bibliographystyle{ieee}
\bibliography{main}
}

\end{document}
